# Supplementary material for: Controllable finite ultra-narrow quality-factor peak in a perturbed Dirac-cone band structure of a photonic crystal slab
Source: arXiv:2104.09818 source file (2021-04-20)
Supplement: Supplementary file 1 [file Supplementary.pdf]

# Supplemental information for Controllable finite ultra-narrow quality-factor peak in a perturbed Dirac-cone band structure of a photonic crystal slab

Alex Y. Song,[1] Akhil Raj Kumar Kalapala,[2] Ricky Gibson,[3] Kevin James Reilly,[4] Thomas Rotter,[4] Sadhvikas Addamane,[4] Haiwen Wang,[5] Cheng Guo,[5] Ganesh Balakrishnan,[4] Robert Bedford,[3] Weidong Zhou,[2] and Shanhui Fan[1,*]

[1]*Department of Electrical Engineering, Stanford University, Stanford, California 94305, USA*

[2]*Department of Electrical Engineering, University of Texas at Arlington, Arlington, Texas 76019, USA*

[3]*Air Force Research Laboratory, Wright-Patterson AFB, Dayton, OH 45433, USA*

[4]*Department of Electrical and Computer Engineering, University of New Mexico, Albuquerque, NM 87131, USA*

[5]*Department of Applied Physics, Stanford University, Stanford, California 94305, USA*

(Dated: 2021-04-20)

## POLES OF THE SCATTERING MATRIX

The band structure and the $Q(\boldsymbol{k})$ functions of a photonic-crystal slab can be directly calculated by computing the poles of the scattering matrix ($S$-matrix) on the complex frequency plane [1]. Here $Q$ is the quality-factor, $\boldsymbol{k} = (k_x, k_y)$ is the in-plane wavevector. The formalism is explained in the following. With light incident at a certain angle $\theta$ from normal, the photonic-crystal slab may generate reflection and transmission. We denote the incident wave amplitudes as $a$ and the outgoing wave amplitudes as $b$. $a$ and $b$ are column vectors which include different polarizations. The scattering matrix $S(\omega, \boldsymbol{k})$ relates the incident wave amplitudes $a$ to the outputs $b$ as

$$b = S(\omega, \boldsymbol{k})a \tag{1}$$

Using the rigorous coupled-wave analysis (RCWA), we can calculate the $S$-matrix with a real wavevector $\boldsymbol{k}$ and a complex frequency $\omega$. With a complex $\omega$, the incident waves, the outgoing waves, and the excited resonances in the photonic-crystal slab are all amplifying or decaying, depending on the sign of the imaginary part of $\omega$. On the complex frequency plane, the frequency $\omega_p$ where the determinant of the $S$-matrix $\det S(\omega, \boldsymbol{k})$ diverges defines a pole of the $S$-matrix. A pole represents a resonance of the structure. In a passive structure, the imaginary frequency of a pole must be positive, if we follow the $e^{i\omega t}$ convention. Hence, by calculating $\det S(\omega, \boldsymbol{k})$ on the upper-half of the complex frequency plane with varying incident angles, we may map out all the entire band structure and the $Q(\boldsymbol{k})$ functions of the structure by locating the poles of the $S$-matrix.

An example is shown in Fig. 1, which corresponds to the same photonic-crystal slab structure studied in the main text in Fig. 2. The circles in Fig. 1a and b are numerical results, obtained from extracting the position of the poles of the $S$-matrix on the complex frequency plane. Several examples of the pole calculation are shown in Fig. 1c-f, which correspond to different incidence angles, i.e. different in-plane wavevectors. Fig. 1c has a zero incidence angle, corresponding to the $\Gamma$ point of the Brillouin zone. There are three poles in Fig. 1c with the same real part of the frequency. One of the pole represents the quadrupole mode and is close to the real axis. The other two poles are degenerate, with a imaginary frequency of $\mathrm{Im} f = 3.8 \times 10^{-4}\, c/l$. As the incidence angle increases, the imaginary frequency of the quadrupole pole starts to increase, while that of one of the dipolar poles decreases. The other dipolar pole stays still. As is observed in Fig. 1d, all three poles

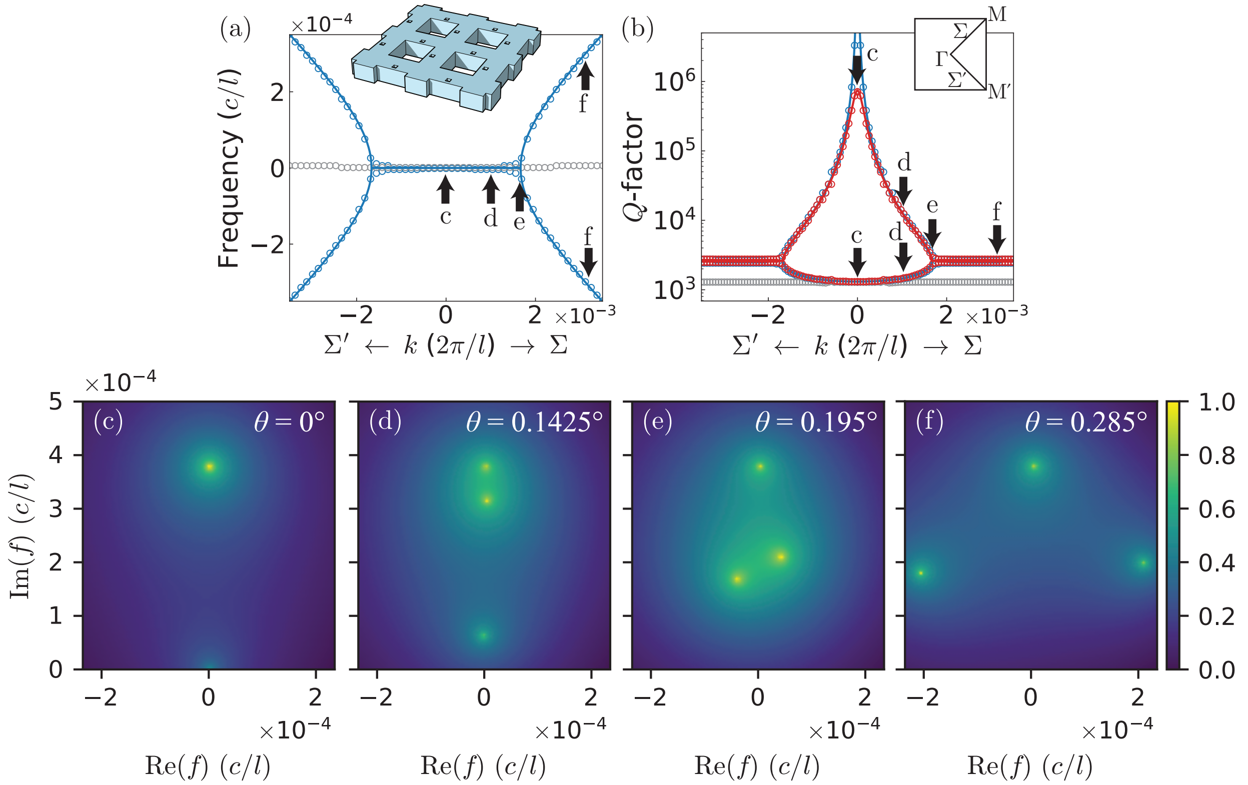


Figure 1. Numerically calculated poles of the $S$-matrix on the complex frequency plane (c-f), the extracted band structure (a), and the $Q(\boldsymbol{k})$ functions (b). (a) and (b) are replotted from Fig. 2 in the main text. The real frequency in (c)-(f) is offset at $0.4906\,c/l$. The real and the imaginary parts of the frequencies of the poles determine the band structure and the $Q$-factor, respectively. The data points obtained from (c)-(f) are marked in (a) and (b) by the black arrows.

maintain their real frequencies initially. The moving quadrupole and the dipolar poles meet near the exceptional point, as is shown in Fig. 1e. Due to the existence of higher-order terms which we ignored in Eq. (1) in the main text, the exact exceptional point is not observed here. As the incidence angle continue to increase, the two moving poles depart in their real frequencies while maintaining their respective imaginary frequencies, as is shown in Fig. 1f. The above dynamics directly translate to the band structure and the $Q(\boldsymbol{k})$ function shown in Fig. 1a and b.

* shanhui@stanford.edu

[1] Alex Y Song, Akhil Raj Kumar Kalapala, Weidong Zhou, and Shanhui Fan, "First-principles simulation of photonic crystal surface-emitting lasers using rigorous coupled wave analysis," Applied Physics Letters **113**, 041106 (2018).
